# Supplementary material for: EdgeMixup: Improving Fairness for Skin Disease Classification and Segmentation
Source: arXiv:2202.13883 source file (2022-02-28)
Supplement: Supplementary file 1 [file appendix.tex]

\section{Appendix}
\label{sec:appendix}

\begin{figure*}[htb!]
\centering
    \centering
    \includegraphics[width=0.49\linewidth]{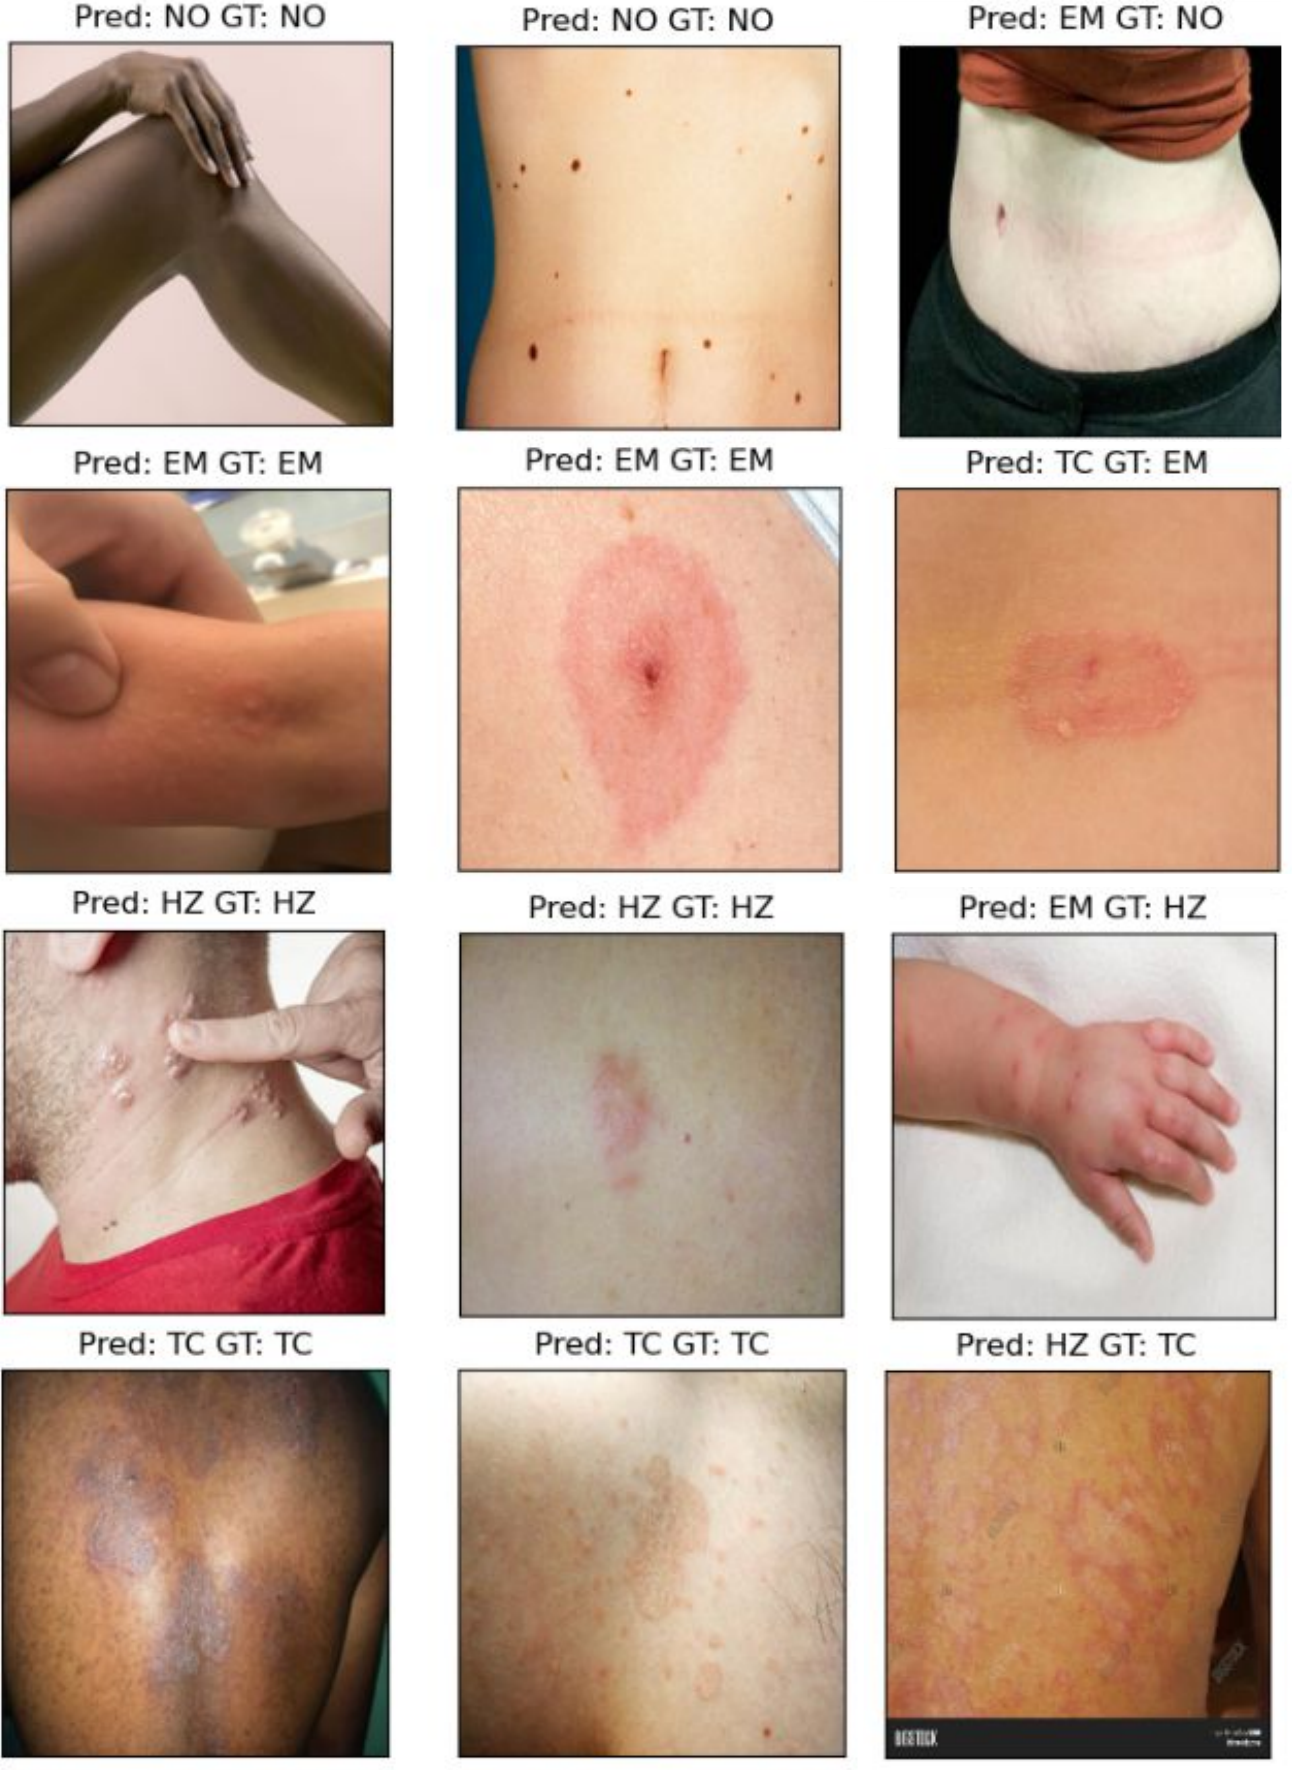}
    \vspace{-0.02\textwidth}
    \caption{Examples of Image+AD model's disease classification predictions (Pred) compared with the known disease (GT) for NO, EM, HZ, and TC.}
    \label{fig:model_clf_examples}
\end{figure*}
\begin{figure}[tb]
    \centering %left, bottom, right top
    \begin{subfigure}{0.49\textwidth}
        \includegraphics[width=\linewidth, trim=0cm 0.18cm 0cm 0cm, clip]{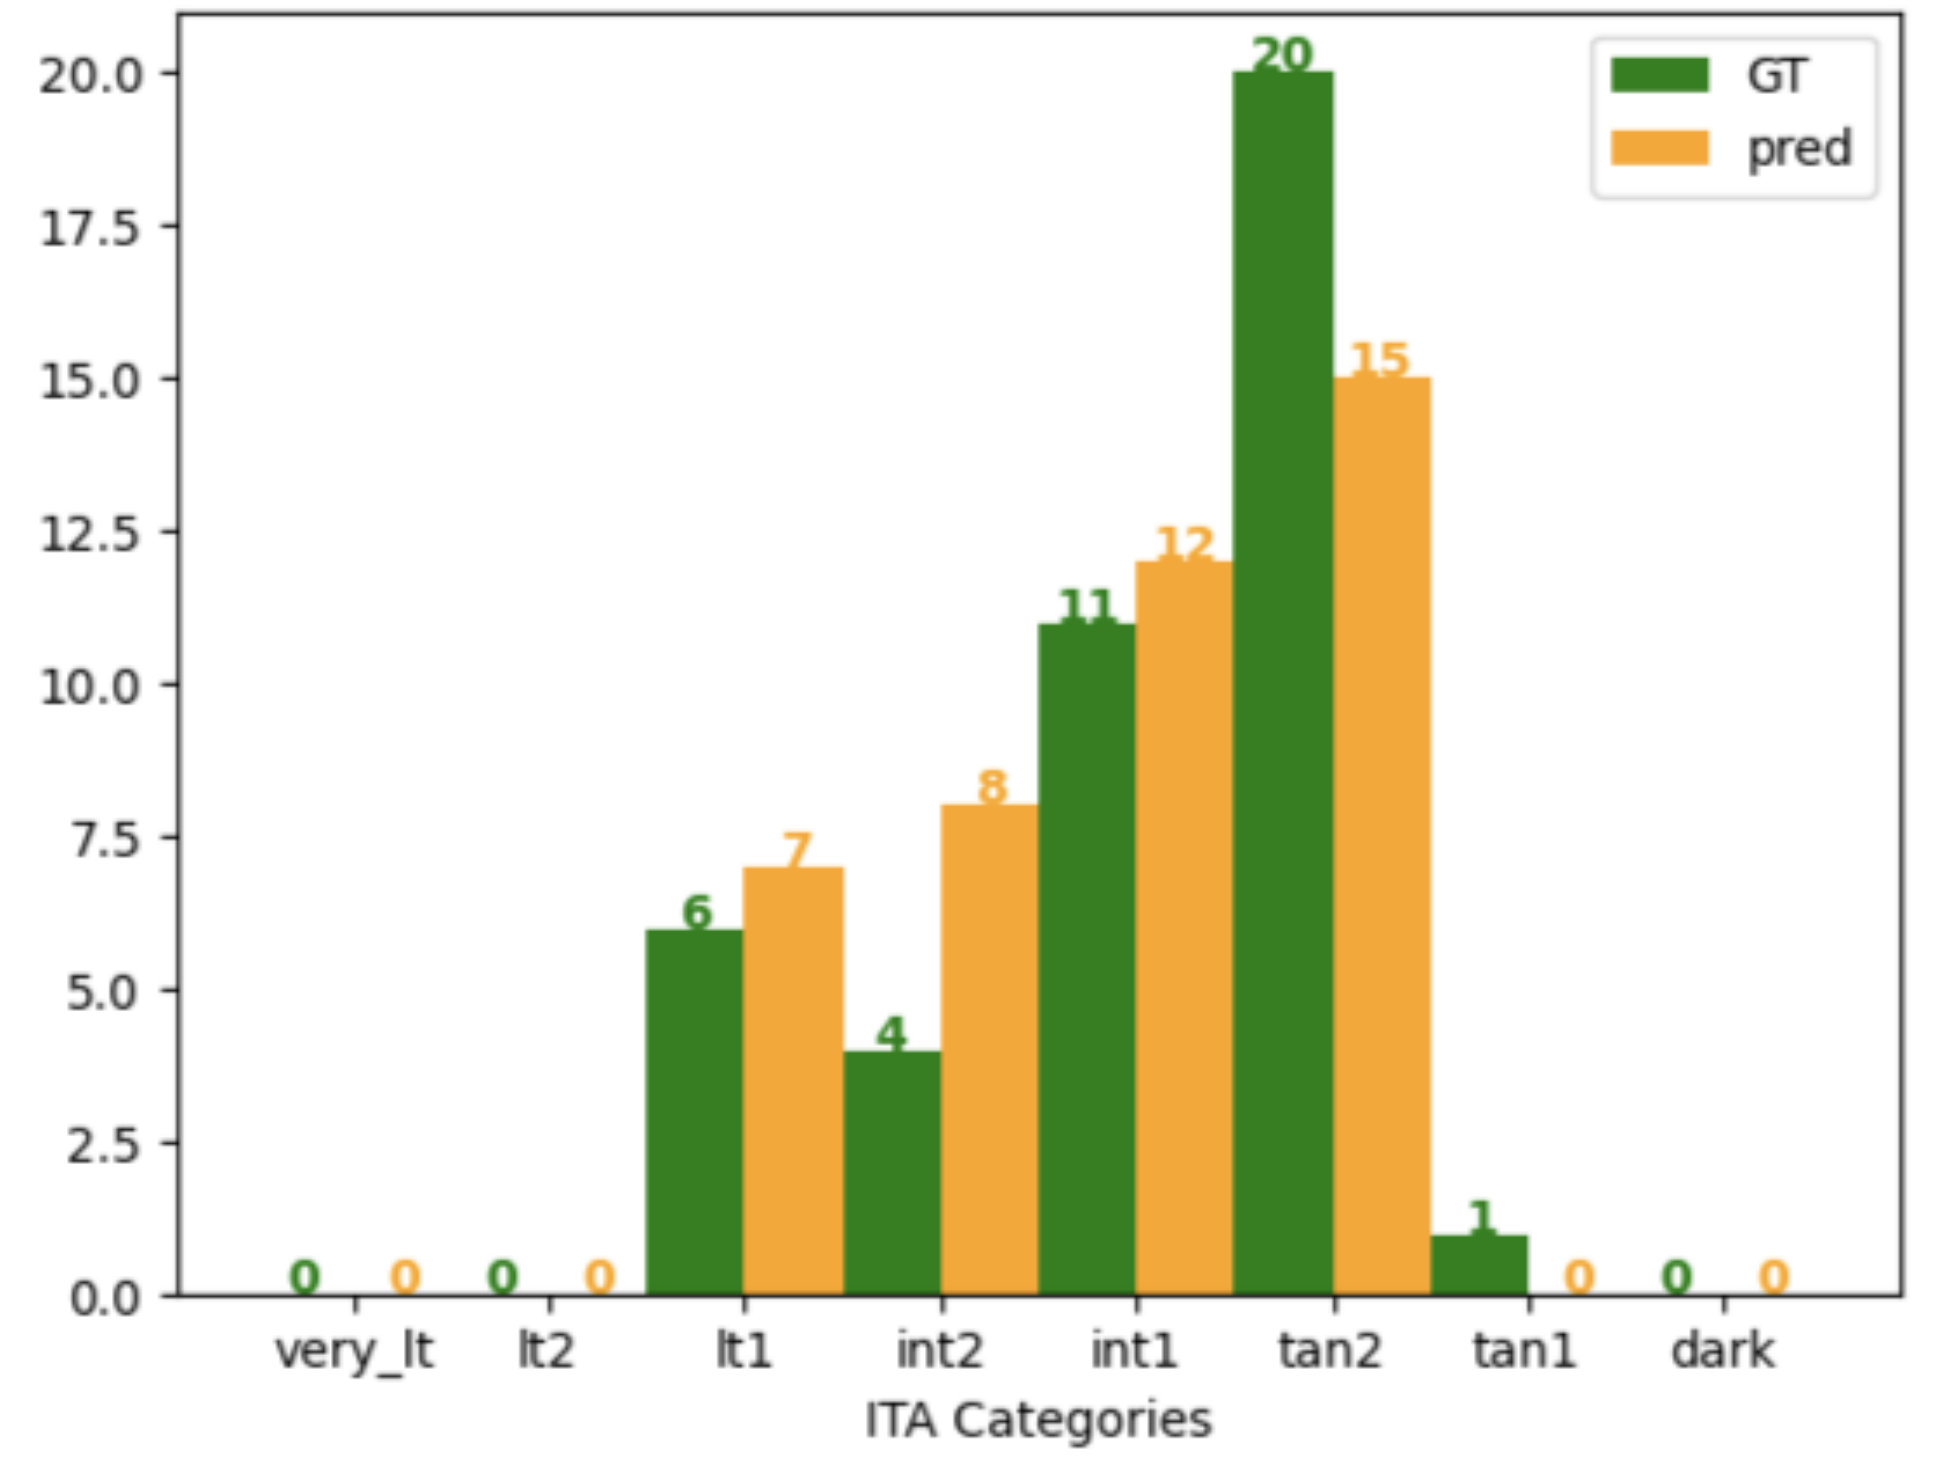}
        \caption{Segmentation}
        \label{fig:seg_test_ita_distribution}
    \end{subfigure}
    \begin{subfigure}{0.49\textwidth}
        \includegraphics[width=\linewidth, trim=3.8cm 8cm 4.1cm 9.1cm, clip]{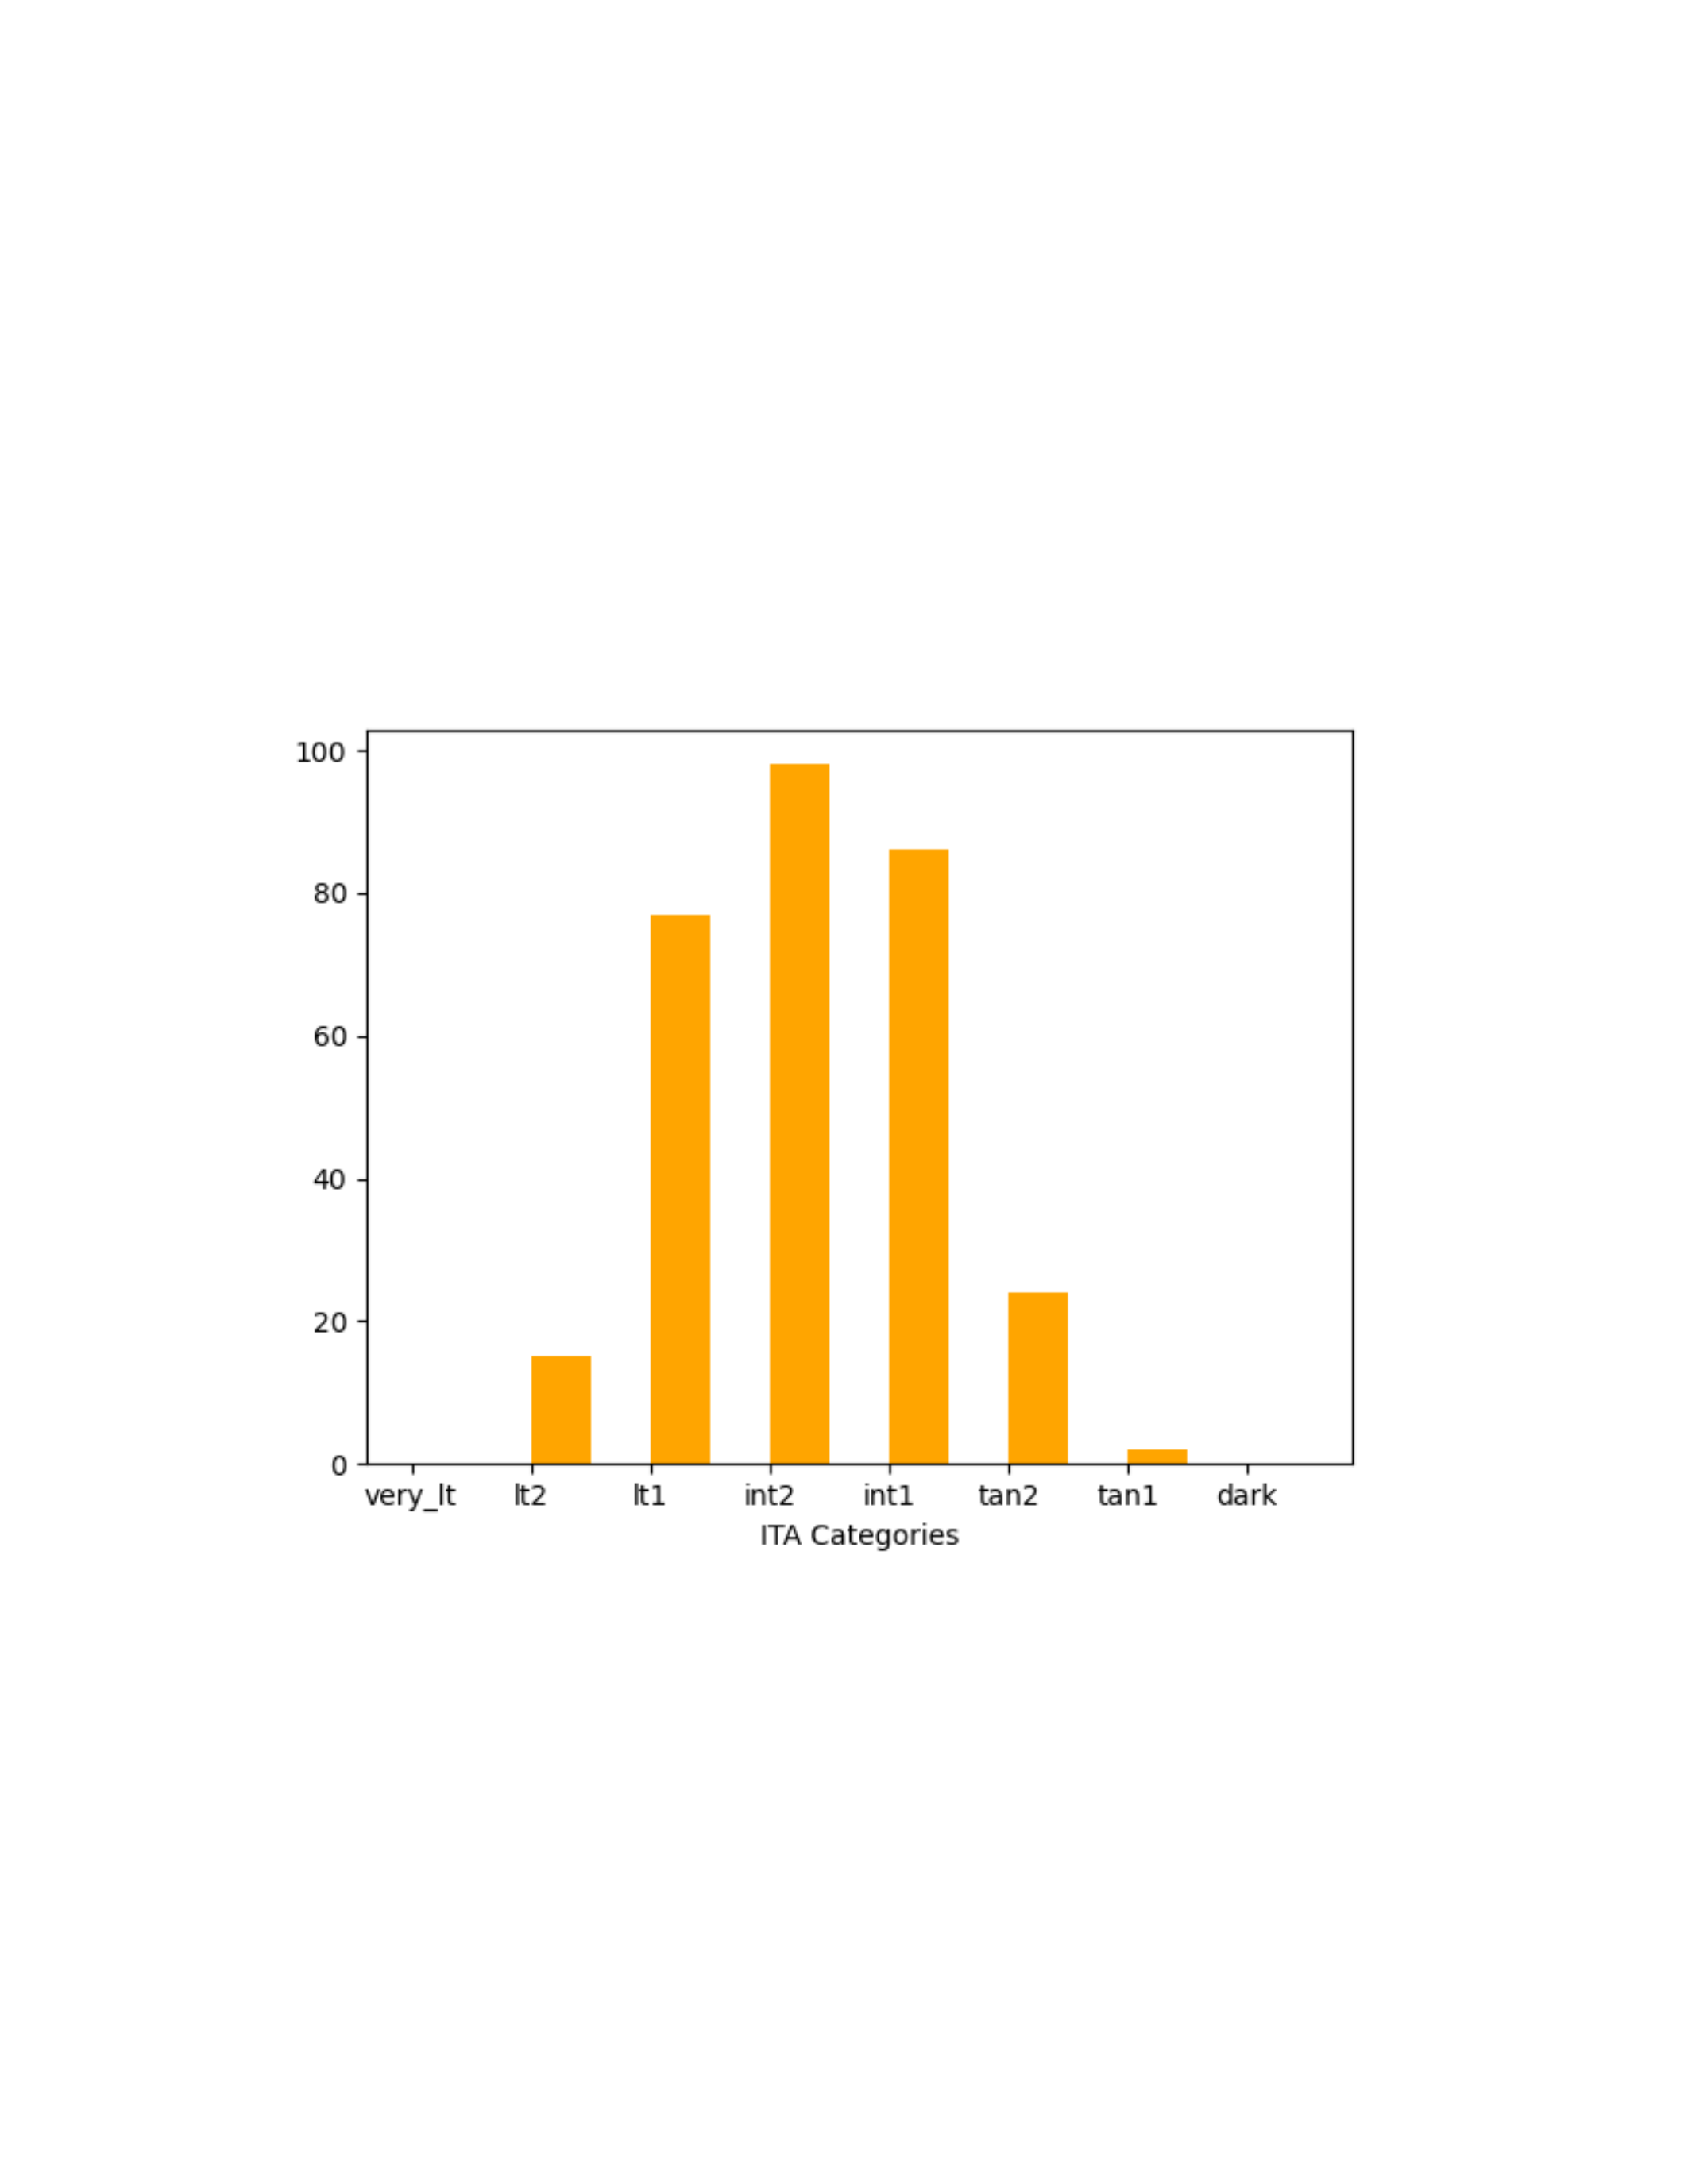}
        \caption{Classification}
        \label{fig:clf_test_ita_distribution}
    \end{subfigure}
    \caption{Test ITA distributions for the (a) segmentation and (b) classification datasets. Predicted (pred) distributions are indicated in orange and known (GT), where available, are indicated in green.}
    \label{fig:dataset_ita_distributions} \vspace{-0.2in}
\end{figure}

\begin{equation}
CAI_{\alpha} = \alpha (acc_{gap}^b - acc_{gap}^d) + (1 - \alpha) (acc^d - acc^b).
\end{equation}

$CAI_{\alpha}: $ Accuracy fairness metric from~\cite{paul2020TARA}.

$\alpha:$ Hyperparameter to balance the importance of a reduction in the accuracy gap and an improvement in accuracy between the baseline $acc^b$ and debiased $acc^d$ methods.

$acc_{gap}^b := \lvert acc_{ls}^b - acc_{ds}^b \rvert:$ Baseline accuracy gap between accuracy on ls and ds samples.

$acc_{gap}^d := \lvert acc_{ls}^d - acc_{ds}^d \rvert:$ Debiased accuracy gap between accuracy on ls and ds samples.

\begin{equation}
CAUCI_{\alpha} = \alpha (AUC_{gap}^b - AUC_{gap}^d) + (1 - \alpha) (AUC^d - AUC^b).
\end{equation}

$CAUCI_{\alpha}:$ AUC fairness metric from~\cite{paul2020TARA}.

$\alpha:$ Hyperparameter to balance the importance of a reduction in the AUC gap and an improvement in AUC between the baseline $AUC^b$ and debiased $AUC^d$ methods. 

$AUC_{gap}^b := \lvert AUC_{ls}^b - AUC_{ds}^b \rvert$ Baseline AUC gap between AUC on ls and ds samples.

$AUC_{gap}^d := \lvert AUC_{ls}^d - AUC_{ds}^d \rvert:$ Debiased AUC gap between AUC on ls and ds samples.
